# Supplementary material for: Decentralized Learning with Approximate Finite-Time Consensus
Source: arXiv:2501.07967 source file (2025-01-14)
Supplement: Supplementary file 1 [file Appendix.tex]

\section{Consensus Error Bound}\label{app:cons-err}
We begin with~\eqref{eq:cons-err-mtau} and bound the consensus error in a similar way to~\cite{koloskova}, by first separating out $\vb_i$ from~\eqref{eq:cons-err-mtau}:
\begin{align}
\expectfi{\norm{\xhat_i}^2} &= \mathbb{E}\big[\big\lVert G_{i:m\tau+1}\xhat_{m\tau}-\mu\sum_{\mathclap{j=m\tau+1}}^{i-1}G_{i:j+1}\hb_{j}-\mu\hb_i\nonumber\\&-\mu\sum_{\mathclap{j=m\tau+1}}^{i-1}G_{i:j+1}\vb_{j} -\mu\vb_i\big\rVert^2 \bigl| \F_{i-1} \big] \\
= \mathbb{E}&\big[\big\lVert G_{i:m\tau+1}\xhat_{m\tau}-\mu\sum_{\mathclap{j=m\tau+1}}^{i-1}G_{i:j+1}\hb_{j}-\mu\hb_i\nonumber\\ -\mu&\sum_{\mathclap{j=m\tau+1}}^{i-1}G_{i:j+1}\vb_{j} \rVert^2 \bigl| \F_{i-1} \big] +\expectfi{\norm{\mu\vb_i}^2}
\end{align}\normalsize
where the cross-terms were removed based on Assumption~\eqref{assump:gradnoise}. The $\hb_i$ term is then split:
\begin{align}
\expectfi{\norm{\xhat_i }^2}& \leq (1+\alpha_1)\mathbb{E}\big[\big\lVert G_{i:m\tau+1}\xhat_{m\tau}\nonumber\\-&\mu\sum_{\mathclap{j=m\tau+1}}^{i-1}G_{i:j+1}\hb_{j}-\mu\sum_{\mathclap{j=m\tau+1}}^{i-1}G_{i:j+1}\vb_{j} \rVert^2 \bigl| \F_{i-1} \big]\nonumber\\ +&\expectfi{\norm{\mu\vb_i}^2} \nonumber\\+&(1+\alpha_1^{-1})\expectfi{\norm{\mu\hb_i}^2}
\end{align}\normalsize
Setting $\alpha_1=\frac{1}{\phi-1}$ for some constant $\phi>1$ that will be defined later:
\begin{align}
\expectfi{\norm{\xhat_i}^2} &\leq \frac{\phi}{\phi-1}\mathbb{E}\big[\big\lVert G_{i:m\tau+1}\xhat_{m\tau}-\mu\sum_{\mathclap{j=m\tau+1}}^{i-1}G_{i:j+1}\hb_{j}\nonumber\\-\mu&\sum_{\mathclap{j=m\tau+1}}^{i-1}G_{i:j+1}\vb_{j} \rVert^2 \bigl| \F_{i-1} \big] +\expectfi{\norm{\mu\vb_i}^2}\nonumber\\+\phi&\expectfi{\norm{\mu\hb_i}^2}
\end{align}\normalsize
We can repeat the process of splitting out $\vb_{i-1}$ and $\hb_{i-1}$ for a constant $\alpha_2$ which we set to $\frac{1}{\phi-2}$ for $\phi>2$:
\begin{align}
\expectfi{\norm{\xhat_i}^2} &\leq \frac{\phi}{\phi-2}\mathbb{E}\big[\big\lVert G_{i:m\tau+1}\xhat_{m\tau}-\mu\sum_{\mathclap{j=m\tau+1}}^{i-2}G_{i:j+1}\hb_{j}\nonumber\\-\mu&\sum_{\mathclap{j=m\tau+1}}^{i-2}G_{i:j+1}\vb_{j} \rVert^2 \bigl| \F_{i-1} \big] +\expectfi{\norm{\mu\vb_i}^2}\nonumber\\ + &\frac{\phi}{\phi-1}\expectfi{\norm{\mu G_i\vb_{i-1}}^2}\nonumber\\+\phi&\expectfi{\norm{\mu\hb_i}^2}+\phi\expectfi{\norm{\mu G_i\hb_{i-1}}^2}
\end{align}
Splitting out the remaining terms in a similar way and using the submultiplicativity of the matrix norm, we are left with:
\begin{align}
    \expectfi{\norm{\xhat_i}^2} &\leq \frac{\phi\epstau^2}{\phi-(2\tau-1)}\norm{\xhat_{m\tau}}^2\nonumber\\+\phi&\mu^2\sum_{\mathclap{j=m\tau+1}}^{i}\expectfi{\norm{\hb_j}^2}\nonumber\\+\mu^2&\sum_{\mathclap{j=m\tau+1}}^{i}~~\frac{\phi}{\phi-(i-j)}\expectfi{\norm{\vb_j}^2} \nonumber
\end{align}\normalsize
for $\phi>2\tau-1$. Applying Lemmas~\eqref{lemma:h_i} and~\eqref{lemma:v_i} and taking the total expectation:
\begin{align}
    \mathbb{E}\norm{\xhat_i}^2 &\leq \epstau^2\left(\frac{\phi\epstau}{\phi-(2\tau-1)}+18\phi\mu^2\delta^2\right)\mathbb{E}\norm{\xhat_{m\tau}}^2\nonumber\\&+9\phi\mu^2K(2\tau-1)B^2+18\phi\mu^2\delta^2\sum_{j=m\tau+1}^{i-1}\norm{\xhat_j}^2\nonumber\\&+\frac{\mu^2(2\tau-1)\phi}{\phi-(2\tau-1)}\sigma^2 \label{eq:cons-err-proof}
\end{align}\normalsize
If $\epstau=0$ then this serves as the upper bound for the consensus error by setting $\phi=2\tau$. Otherwise, we can apply Eq.~\eqref{eq:cons-err-proof} for ${\mathbb{E}\norm{\xhat_{i-1}}^2}$ in the summation term, and then again for ${\mathbb{E}\norm{\xhat_{(i-2)}}^2}$ and so on until the bound is expressed entirely in terms of ${\mathbb{E}\norm{\xhat_{m\tau}}^2}$. Setting ${\phi=\frac{2\tau(1+\epstau)}{1-\epstau}}$, ${\mu\leq\frac{1}{12\delta^2}\sqrt{\frac{1-\epstau}{\tau(2\tau-1)(1+\epstau)}}}$ and using the fact that ${\left(1+\frac{\beta}{n}\right)^n\leq 1+2\beta}$ for ${0\leq\beta\leq1}$, we arrive at the final bound for the consensus error in Theorem~\eqref{thm:cons-bound}.\\
